# Supplementary material for: Efimov States of Strongly Interacting Photons
Source: arXiv:1709.01955 source file (2017-09-28)
Supplement: Supplementary file 1 [file RydEfimov_supp.pdf]

# Supplemental Material to the Manuscript: "Efimov States of Strongly Interacting Photons"

## I. TWO-BODY SCATTERING WITH ANISOTROPIC MASS

In this section we compare the scaling of the $T$-matrix elements with energy for the higher-partial waves in the two-body problem with an anisotropic mass to the Born approximation.

The Schrödinger equation for the wavefunction of two dark-state polaritons (branch $\mu = D$) with identical anisotropic masses in the rescaled coordinates defined in the main text is

$$-\frac{\tilde{\nabla}^2\psi}{m} + U(\tilde{r},\tilde{\theta})\psi = E\psi, \tag{S1}$$

$$U(\tilde{r},\tilde{\theta}) = -\frac{\alpha/\bar{\chi}[2\epsilon_D(\boldsymbol{q}_0)]}{1+\frac{\tilde{r}^6}{r_0^6}\left(1+\frac{\cos^2\tilde{\theta}\cos 2\beta}{\sin^2\beta}\right)^3}, \tag{S2}$$

$$\bar{\chi}(\omega) = \frac{\Delta-\omega/2-\frac{\Omega^2}{\Delta-\omega}}{\omega(\Delta-\omega/2)+2\Omega^2},\ \alpha \approx |S_D^{\boldsymbol{q}_0}|^4, \tag{S3}$$

$$|S_\mu^{\boldsymbol{q}}|^2 = \frac{\Omega^2}{\Omega^2+\epsilon_\mu(\boldsymbol{q})^2}, \tag{S4}$$

where $\boldsymbol{q}_0$ is the incoming momentum of the two dark-state polaritons and $S_\mu^{\boldsymbol{q}}$ is the overlap of the single polariton eigenstate on branch $\mu$ with momentum $\boldsymbol{q}$ with the Rydberg state. Expanding the wavefunction in spherical harmonics and dropping the tildes over the rescaled coordinates

$$\psi = \frac{1}{r}\sum_{\ell,m} Y_{\ell m}(\theta,\phi) f_{\ell m}(r), \tag{S5}$$

we arrive at the radial Schrödinger equation

$$-\frac{f''_{\ell m}}{m} + \frac{\ell(\ell+1)}{mr^2}f_{\ell m} + \sum_{\ell'} U_{\ell\ell'}^{(m)}(r) f_{\ell' m} = E f_{\ell m}, \tag{S6}$$

$$U_{\ell\ell'}^{(m)}(r) = 2\pi\int_0^\pi \sin\theta d\theta\, Y_{\ell m}^*(\theta,\phi)U(r,\theta)Y_{\ell' m}(\theta,\phi), \tag{S7}$$

with the boundary conditions [S1]

$$\lim_{r\to 0} f_{\ell m}^{\ell' m}(r) = 0, \tag{S8}$$

$$\lim_{r\to\infty} f_{\ell m}^{\ell' m}(r) = \delta_{\ell\ell'}e^{-i(kr-\frac{\ell'\pi}{2})} - S_{\ell\ell'}^{(m)}e^{i(kr-\frac{\ell'\pi}{2})}. \tag{S9}$$

Here $k=\sqrt{mE}$ and $S_{\ell\ell'}^{(m)}$ is the multi-channel $S$-matrix, which has to be found self-consistently.

In the first Born approximation the scattering amplitude defined in Eq. (9) of the main text takes the form

$$f(\hat{k}_i,\hat{k}_f) = -\frac{1}{2\pi}\int d^3r e^{i\boldsymbol{k}_i\cdot\boldsymbol{r}}U(r,\theta)e^{-\boldsymbol{k}_f\cdot\boldsymbol{r}}. \tag{S10}$$

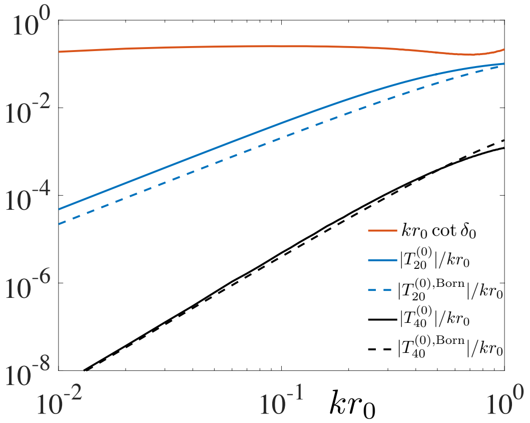


FIG. S1: (a) Scaling of $T$-matrix elements as a function of $k=\sqrt{mE}$. Near threshold, the scattering is dominated by the diagonal $s$-wave component $S_{00}^{(0)} = e^{i\delta_0(k)}$, which defines the scattering length via $k\cot\delta_0 = -1/a + O(k^2)$. Here we took $\sqrt{mU(0)}r_0 = 2.2$ and $m_\perp/m_z = 20$.

Using the expansion of $e^{i\boldsymbol{k}\cdot\boldsymbol{r}}$ into spherical harmonics, this equation directly implies that

$$T_{\ell\ell'}^{(m),\mathrm{Born}} = -k\Gamma_{\ell\ell'}^{(m)}, \tag{S11}$$

$$\Gamma_{\ell\ell'}^{(m)} = -4\int r^2 dr j_\ell(kr)j_{\ell'}(kr)U_{\ell\ell'}^{(m)}(r), \tag{S12}$$

where $j_\ell(x)$ are spherical Bessel functions. For an interaction potential that dies off as $1/r^s$, $T_{\ell\ell'}^{(m),\mathrm{Born}}$ has the scaling given in Eq. (10) of the main text. We have verified these scalings for the higher partial wave $S$-matrix elements using numerical solutions of the radial Schrödinger equation. An example is shown in Fig. S1(a) for the $s$-wave channel with a large mass ratio of $m_\perp/m_z = 20$. In Fig. 2(c) of the main text we obtained the scattering length through numerical solutions of the $S$-matrix including the $\ell = 0$ and $\ell = 2$ partial wave channels. We further verified that including the $\ell = 4$ channel had a negligible effect on the position of the $s$-wave scattering resonances, which is consistent with the perturbative analysis in Sec. III.

## II. SCALING OF THREE-BODY LOSS RATE

In this section, we derive the scaling of the three-body loss rate near the EIT resonance for large values of the interaction parameter $\phi = g^2 r_b/c\Delta = \mathrm{OD}_b\gamma/\Delta$, where $\mathrm{OD}_b$ is the optical depth per blockade radius.

From the optical theorem, the three-body loss appears as an imaginary contribution to the self-energy

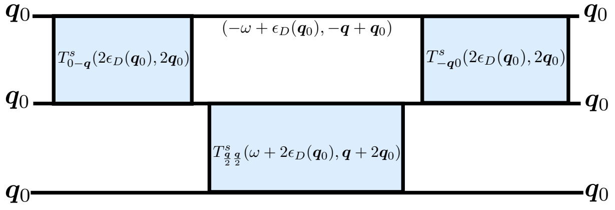


FIG. S2: One-loop contribution to the three-body $T$-matrix with all incoming and outgoing states dark-state polaritons at the same momentum. The imaginary part of this diagram gives the lowest order contribution to the three-body loss rate.

of three dark-state polaritons [S2]. Thus we can find the lowest order contribution to the three-body loss rate in the two-body $T$-matrix by evaluating the imaginary part of the diagram in Fig. S2, which contains a single loop. In this diagram the shaded boxes represent the symmetrized two-particle $T$-matrix $T^s_{\boldsymbol{k}\boldsymbol{k}'}(\omega, K) = [T_{\boldsymbol{k}\boldsymbol{k}'}(\omega, \boldsymbol{K}) + T_{\boldsymbol{k}-\boldsymbol{k}'}(\omega, \boldsymbol{K})]/2$, where $\omega$ and $\boldsymbol{K} = \boldsymbol{q}_1 + \boldsymbol{q}_2$ are the total energy and momentum of the incoming polaritons with momenta $\boldsymbol{q}_{1,2}$, respectively, $\boldsymbol{k} = (\boldsymbol{q}_1 - \boldsymbol{q}_2)/2$ is the incoming relative momentum of the two polaritons, and $\boldsymbol{k}'$ is the outgoing relative momentum. The solid lines are the time-ordered, non-interacting Green's function for a single Rydberg state

$$g^{\boldsymbol{q}}_s(\omega) = \sum_\mu \frac{|S^{\boldsymbol{q}}_\mu|^2}{\omega - \epsilon_\mu(\boldsymbol{q}) + i\epsilon}, \tag{S13}$$

where $S^{\boldsymbol{q}}_\mu$ is the overlap of the single polariton eigenstate on branch $\mu$ with momentum $\boldsymbol{q}$ with the Rydberg state. Using these Feynman rules and performing the integral over the virtual frequency $\omega$, the diagram in Fig. S2 evaluates to

$$\int \frac{d^3q}{8\pi^3} \sum_{\mu,\nu,\gamma} |S^{\boldsymbol{q}_0-\boldsymbol{q}}_\mu|^2 |S^{\boldsymbol{q}_0+\boldsymbol{q}}_\nu|^2 |S^{\boldsymbol{q}_0+\boldsymbol{q}}_\gamma|^2 \frac{T^s_{0-\boldsymbol{q}}(2\epsilon_D(\boldsymbol{q}_0), 2\boldsymbol{q}_0) T^s_{\frac{\boldsymbol{q}}{2}\frac{\boldsymbol{q}}{2}}(3\epsilon_D(\boldsymbol{q}_0) - \epsilon_\mu(\boldsymbol{q}_0 - \boldsymbol{q}), 2\boldsymbol{q}_0 + \boldsymbol{q}) T^s_{-\boldsymbol{q}0}(2\epsilon_D(\boldsymbol{q}_0), 2\boldsymbol{q}_0) |S^{\boldsymbol{q}_0}_D|^6}{[2\epsilon_D(\boldsymbol{q}_0) - \epsilon_\mu(\boldsymbol{q}_0 - \boldsymbol{q}) - \epsilon_\nu(\boldsymbol{q}_0 + \boldsymbol{q})][2\epsilon_D(\boldsymbol{q}_0) - \epsilon_\mu(\boldsymbol{q}_0 - \boldsymbol{q}) - \epsilon_\gamma(\boldsymbol{q}_0 + \boldsymbol{q})]}. \tag{S14}$$

Neglecting the contribution from two-body poles, which were shown to be strongly suppressed in this system [S3], the only genuine three-body poles in the integrand appear in $T^s_{\frac{\boldsymbol{q}}{2}\frac{\boldsymbol{q}}{2}}(3\epsilon_D(\boldsymbol{q}_0) - \epsilon_\mu(\boldsymbol{q}_0 - \boldsymbol{q}), 2\boldsymbol{q}_0 + \boldsymbol{q})$. When there are deep two-body bound states, the pole will appear at low virtual momentum. Evaluating the integral over this pole will give the lowest order contribution to the three-body recombination rate. In the absence of two-body bound states, the only poles in $T^s_{\frac{\boldsymbol{q}}{2}\frac{\boldsymbol{q}}{2}}(3\epsilon_D(\boldsymbol{q}_0) - \epsilon_\mu(\boldsymbol{q}_0 - \boldsymbol{q}), 2\boldsymbol{q}_0 + \boldsymbol{q})$ arise from the kinematically allowed loss processes into free polaritons discussed in the main text, which occur at large $q_z$.

To more explicitly demonstrate the exponential suppression of these contributions we note that the two-body $T$-matrix can be found from the Lippmann-Schwinger equation for Rydberg polaritons generalized to include the transverse momentum [S3]

$$T_{\boldsymbol{k}\boldsymbol{k}'}(\omega, \boldsymbol{K}) = V_{\boldsymbol{k}-\boldsymbol{k}'} + \int \frac{d^3q}{(2\pi)^3} V_{\boldsymbol{k}-\boldsymbol{q}} g^{\boldsymbol{q}}_{ss}(\omega, \boldsymbol{K}) T_{\boldsymbol{q}\boldsymbol{k}'}(\omega, \boldsymbol{K}), \tag{S15}$$

$$g^{\boldsymbol{q}}_{ss}(\omega, \boldsymbol{K}) = \sum_{\mu,\nu} \frac{|S^{\boldsymbol{K}/2+\boldsymbol{q}}_\mu|^2 |S^{\boldsymbol{K}/2-\boldsymbol{q}}_\nu|^2}{\omega - \epsilon_\mu(\boldsymbol{K}/2 + \boldsymbol{q}) - \epsilon_\nu(\boldsymbol{K}/2 - \boldsymbol{q}) + i\epsilon}, \tag{S16}$$

where $g^{\boldsymbol{q}}_{ss}(\omega, \boldsymbol{K})$ is the non-interacting, time-ordered Green's function for two Rydberg states.

For relative momenta $q_z$ much larger than $g^2/c\Delta$, $g^{\boldsymbol{q}}_{ss}(\omega, \boldsymbol{K})$ saturates to the constant

$$\bar{\chi}(\omega) = \lim_{|q_z| \to \infty} g^{\boldsymbol{q}}_{ss}(\omega, \boldsymbol{K}) \tag{S17}$$

which implies that the $T$-matrix for large longitudinal momentum transfers approaches $T_{\boldsymbol{k}\boldsymbol{k}'}(\omega, \boldsymbol{K}) \approx U_{\boldsymbol{k}-\boldsymbol{k}'}/\alpha$, where $U_{\boldsymbol{k}} = \int d^3r e^{i\boldsymbol{k}\cdot\boldsymbol{r}} U(\boldsymbol{r})$ and $U(\boldsymbol{r})$ is defined in Eq. (1) of the main text.

From the expressions for $v_g$ and $m_{z,\perp}$ in the main text (Eqs. (4)-(6)) we see that near the EIT resonance (i.e., $\epsilon_\mu(\boldsymbol{q}) \ll \Delta$) and in the regime $g \gg |\Delta|$ with $|\Delta| \gg \Omega$, the typical variations in the dispersion with respect to $q_z$ occur on momentum scales $g^2/c\Delta$. This implies that, in the large $\phi = g^2 r_b/c\Delta$ limit, $r_b^{-1}$ is a small momentum scale with respect to the polariton dispersion. From the analysis in the main text we know that, in the absence of two-body bound states, the three-body resonances in Eq. (S14) are associated with large virtual momentum $q_z$. This implies that the three-body loss will be exponentially suppressed by the term $[T^s_{0\boldsymbol{q}}(2\epsilon_D(\boldsymbol{q}_0), 2\boldsymbol{q}_0)]^2 \approx |U_{\boldsymbol{q}}|^2/\alpha^2$ evaluated at the resonant values of $\boldsymbol{q}$. Near the inflection point there is an additional suppression of the three-body loss from the overlap factor with the incoming and outgoing dark-state polaritons $|S^{\boldsymbol{q}_0}_D|^6 \approx \Omega^2/\Delta^2$.

## III. PERTURBATIVE INCLUSION OF MASS ANISOTROPY

In this section, we introduce an approximation method that includes the effect of the anisotropic mass by treating the coupling to the higher-partial waves in the rescaled coordinates perturbatively.

In the rescaled coordinates, the multichannel potential matrix $U_{\ell\ell'}(r)$ [see Eq. (S6)] fully describes anisotropic interactions on the two-body level. In principle, a numerically exact treatment of the three-body scattering problem requires this multichannel two-body potential, including all partial waves. However, we can most simply describe the qualitative affect of anisotropic interactions on important three-body physics, like the Efimov effect, using a single-channel two-body potential. To this end we use a two-body model potential $U'(r)$ that perturbatively includes the affect of anisotropic interactions.

For isotropic interactions the potential matrix $U_{\ell\ell'}(r)$ becomes diagonal, and we can fully describe low-energy scattering using only the $s$-wave ($\ell = 0$) potential. We find corrections to this potential due to anisotropic interactions using second-order perturbation theory in an approximation that only captures s-wave resonances [S1],

$$U'(r) = U_{00}(r) - \sum_{\ell \neq 0}^{\ell_{\max}} \frac{U_{0\ell}^2(r)}{U_{\ell\ell}(r) - U_{00}(r)}, \tag{S18}$$

where the value $\ell_{\max}$ identifies the highest partial wave included in the model potential $U'(r)$. This potential can be numerically converged by taking the limit $\ell_{\max} \to \infty$.

The terms of the sum on the right hand side of equation (S18) decrease rapidly with increasing $l$. We define each term as

$$\Delta U'_\ell(r) = -\frac{U_{0\ell}^2(r)}{U_{\ell\ell}(r) - U_{00}(r)}. \tag{S19}$$

We show each non-zero term from $\ell = 0 - 6$ in Fig. S3, where only even partial waves couple to the $s$-wave channel. For $\ell > 6$ each term is essentially zero for all $r$ on this scale.

In order to study Efimov physics we tune the depth of our model potential $U'(0)$ such that a two-body bound state resides at zero energy and the scattering length of this potential diverges. For each choice of $\ell_{\max}$ this resonant depth is slightly different. Table I shows these depths for a mass ratio $m_\perp/m_z = 10$. We see that the depth converges quickly as a function of $\ell_{\max}$ and that the addition of $\Delta U'_6(r)$ makes less than a 0.1% change in the depth. Therefore, we neglect contributions to $U'(r)$ from channels of partial-wave character greater than $\ell = 6$. Furthermore, the position of the first scattering resonance computed using this approximation agrees with the non-perturbative calculations presented in Fig. 2(c) of the main text and in Sec. I. We choose $\ell_{\max} = 6$ to construct the model potential $U'(r)$, and we compute three-body potentials using this model. Although an accurate description of the three-body physics requires the full treatment of the anisotropic character of the two-body interactions, our simple model is able to qualitatively describe the dependence of Efimov physics on the strength of the anisotropy (see, for instance, Ref. [S4])

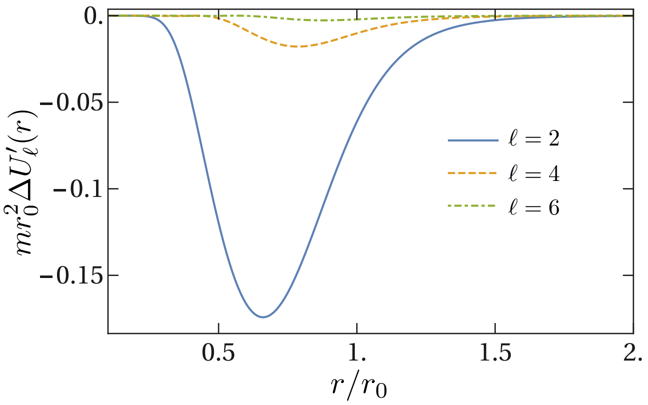


FIG. S3: Each non-zero term $\Delta U'_\ell(r)$ in the perturbative correction to the potential $U_{00}(r)$ due to anisotropic interactions. We show the range $\ell = 0 - 6$. The mass ratio $m_\perp/m_z = 10$.

TABLE I: The depth of the potential $U'(r)$ that supports a zero-energy bound state, for each value of $\ell_{\max}$. The mass ratio $m_\perp/m_z = 10$.

| $\ell_{\max}$ | $\sqrt{-mU'(0)}r_0$ |
|---|---|
| 0 | 2.3339 |
| 2 | 2.2705 |
| 4 | 2.2645 |
| 6 | 2.2635 |


[S1] J. L. Bohn, M. Cavagnero, and C. Ticknor, *Quasi-universal dipolar scattering in cold and ultracold gases*, New J. Phys. **11**, 055039 (2009).

[S2] E. Braaten and H. W. Hammer, *Three-Body Recombination into Deep Bound States in a Bose Gas with Large Scattering Length*, Phys. Rev. Lett. **87**, 160407 (2001).

[S3] P. Bienias, S. Choi, O. Firstenberg, M. F. Maghrebi, M. Gullans, M. D. Lukin, A. V. Gorshkov, and H. P. Büchler, *Scattering resonances and bound states for strongly interacting Rydberg polaritons*, Phys. Rev. A **90**, 053804 (2014).

[S4] Y. Wang, J. P. D'Incao, and C. H. Greene, *Efimov effect for three interacting bosonic dipoles*, Phys. Rev. Lett. **106**, 233201 (2011).
